# Supplementary material for: A multi-task learning-based optimization approach for finding diverse sets of material microstructures with desired properties and its application to texture optimization
Source: arXiv:2111.00916 source file (2022-03-23)
Supplement: Supplementary file 1 [file Appendix.tex]

\section{Parameter ranges for BCC rolling texture generation}
\label{sec:appendix_A}

Table \ref{tab:delannay_parameter_ranges} shows the ranges of the parameters $P_i$.

\begin{table}[h!]
	\caption{Parameter ranges for $P_i$}
	\label{tab:delannay_parameter_ranges}
	\begin{center}
		\begin{tabular}{l | c c c c c c c }
			rel. intensity & $P_1$ & $P_2$ & $P_3$ & $P_4$ & $P_5$ & $P_6$ & \\
			\hline
			min & $1/6$ & $1/6$ & $1/6$ & $0$ & $1/6$ & $1/6$ & \\
			max & $1/3$ & $2/3$ & $2/3$ & $1/3$ & $1$ & $1$ & \\
			unit & - & - & - & - & - & - & 
			\vspace{2 mm} \\
			thickness & $P_7$ & $P_8$ & $P_9$ & $P_{10}$ & $P_{11}$ & $P_{12}$ & $P_{13}$ \\
			\hline
			min & $5/3$ & $5/3$ & $5/3$ & $5/3$ & $5/3$ & $5/3$ & $5/3$ \\
			max & $45/3$ & $35/3$ & $35/3$ & $30/3$ & $30/3$ & $30/3$ & $35/3$ \\
			unit & $^\circ$ & $^\circ$ & $^\circ$ & $^\circ$ & $^\circ$ & $^\circ$ & $^\circ$ 
			\vspace{2 mm} \\
			shift & $P_{14}$ & $P_{15}$ & $P_{16}$ & $P_{17}$ & $P_{18}$ & $P_{19}$ & \\
			\hline
			min & $-5$ & $-10$ & $-10$ & $-5$ & $-10$ & $-10$ & \\
			max & $10$ & $10$ & $5$ & $10$ & $10$ & $10$ &  \\
			unit & $^\circ$ & $^\circ$ & $^\circ$ & $^\circ$ & $^\circ$ & $^\circ$ & 
		\end{tabular}
	\end{center}
\end{table}

\section{Results inverse}

\subsection{Siamese-MTL}
\label{subsec:Results-Siamese-MTL}
regression: r2, corrc, mae e, mae r
rekonstruktion: rekon-loss.
reachability: reach-loss.
distance preserve: r2, corrc, mae.

\begin{table}[h]
	\label{tab:Results-of-Simaese-MTL-Regression}
	\begin{center}
		\begin{tabular}{| l | l | l | l | l |}
			\hline		
			LF & R2 		& Corrc 	& MAE-E 	& MAE-R \\
			\hline
			20 & 00.0000 	& 00.0000 	& 0.0000	& 0.0000\\
			18 & 00.0000 	& 00.0000 	& 0.0000	& 0.0000\\
			16 & 00.0000 	& 00.0000 	& 0.0000	& 0.0000\\
			14 & 00.0000 	& 00.0000 	& 0.0000	& 0.0000\\
			12 & 00.0000 	& 00.0000 	& 0.0000	& 0.0000\\
			10 & 00.0000 	& 00.0000 	& 0.0000	& 0.0000\\
			 8 & 00.0000 	& 00.0000 	& 0.0000	& 0.0000\\
			 6 & 00.0000 	& 00.0000 	& 0.0000	& 0.0000\\								
			 4 & 00.0000 	& 00.0000 	& 0.0000	& 0.0000\\									
			\hline			 
		\end{tabular}
	\end{center}
	\caption{Simaese-MTL: Regression Results}
\end{table}

\begin{table}[h]
	\label{tab:Results-of-Simaese-MTL-Real-Texture}
	\begin{center}
		\begin{tabular}{| l | l | l |}
			\hline		
			LF & MAE-E 	& MAE-R \\
			\hline
			20 & 0.0000	& 0.0000\\
			18 & 0.0000	& 0.0000\\
			16 & 0.0000	& 0.0000\\
			14 & 0.0000	& 0.0000\\
			12 & 0.0000	& 0.0000\\
			10 & 0.0000	& 0.0000\\
			 8 & 0.0000	& 0.0000\\
			 6 & 0.0000	& 0.0000\\								
			 4 & 0.0000	& 0.0000\\									
			\hline			 
		\end{tabular}
	\end{center}
	\caption{Simaese-MTL: Real Texture}
\end{table}

\begin{table}[h]
	\label{tab:Results-of-Simaese-MTL-Preserve}
	\begin{center}
		\begin{tabular}{| l | l | l | l |}
			\hline		
			LF & R2 		& Corrc 	& MAE 		\\
			\hline
			20 & 00.0000 	& 00.0000 	& 0.0000	\\
			18 & 00.0000 	& 00.0000 	& 0.0000	\\
			16 & 00.0000 	& 00.0000 	& 0.0000	\\
			14 & 00.0000 	& 00.0000 	& 0.0000	\\
			12 & 00.0000 	& 00.0000 	& 0.0000	\\
			10 & 00.0000 	& 00.0000 	& 0.0000	\\
			 8 & 00.0000 	& 00.0000 	& 0.0000	\\
			 6 & 00.0000 	& 00.0000 	& 0.0000	\\								
			 4 & 00.0000 	& 00.0000 	& 0.0000	\\									
			\hline			 
		\end{tabular}
	\end{center}
	\caption{Simaese-MTL: Preserve Results}
\end{table}

\begin{table}[h]
	\label{tab:Results-of-Simaese-MTL-Recon}
	\begin{center}
		\begin{tabular}{| l | l |}
			\hline		
			LF & Recon 	\\
			\hline
			20 & 0.0000 \\
			18 & 0.0000	\\
			16 & 0.0000	\\
			14 & 0.0000	\\
			12 & 0.0000	\\
			10 & 0.0000	\\
			 8 & 0.0000	\\
			 6 & 0.0000	\\								
			 4 & 0.0000	\\									
			\hline			 
		\end{tabular}
	\end{center}
	\caption{Simaese-MTL: Reconstruction}
\end{table}

%\begin{figure}%
%  \centering
%  \subfloat[][]{\includegraphics[width=0.80\linewidth]{Figures/Target-region-1-e00-e90}}%
%  \qquad
%  \subfloat[][]{\includegraphics[width=0.80\linewidth]{Figures/Target-region-1-r00-r90}}%
%  \caption{Target region for the (a) E-values and (b) $r$-values  at 0 and 90 degree to rolling direction. It indicates the microstructures from the dataset (blue %density distribution),  the target region (red square), and the baseline consisting of microstructures within the target region (green dots).\textbf{Grafik OK?}}
%  \label{img:Target-region-1-e-and-r}
%\end{figure}

\begin{figure}
	\centering
  	\includegraphics[width=0.95\linewidth]{Figures/Structure-Space}
	\caption{Structure-Space}
	\label{fig:Structure-Space}
\end{figure}

\begin{figure}
	\centering
  	\includegraphics[width=0.95\linewidth]{Figures/Generated-microstructure-compare-poleplots-v1}
	\caption{Generated-microstructure-compare-poleplots-v1}
	\label{fig:Generated-microstructure-compare-poleplots-v1}
\end{figure}

\begin{figure}
	\centering
  	\includegraphics[width=0.95\linewidth]{Figures/Generated-microstructure-compare-poleplots-v2}
	\caption{Generated-microstructure-compare-poleplots-v2}
	\label{fig:Generated-microstructure-compare-poleplots-v2}
\end{figure}

\begin{figure}
	\centering
  	\includegraphics[width=0.95\linewidth]{Figures/Model-Layers}
	\caption{Model-Layers}
	\label{fig:Model-Layers}
\end{figure}
